# Supplementary material for: Statistical mechanical properties of sequence space determine the efficiency of the various algorithms to predict interaction energies and native contacts from protein coevolution
Source: arXiv:1902.01155 source file (2019-02-04)
Supplement: Supplementary file 1 [file SuppMat.pdf]

**Supplementary Materials**

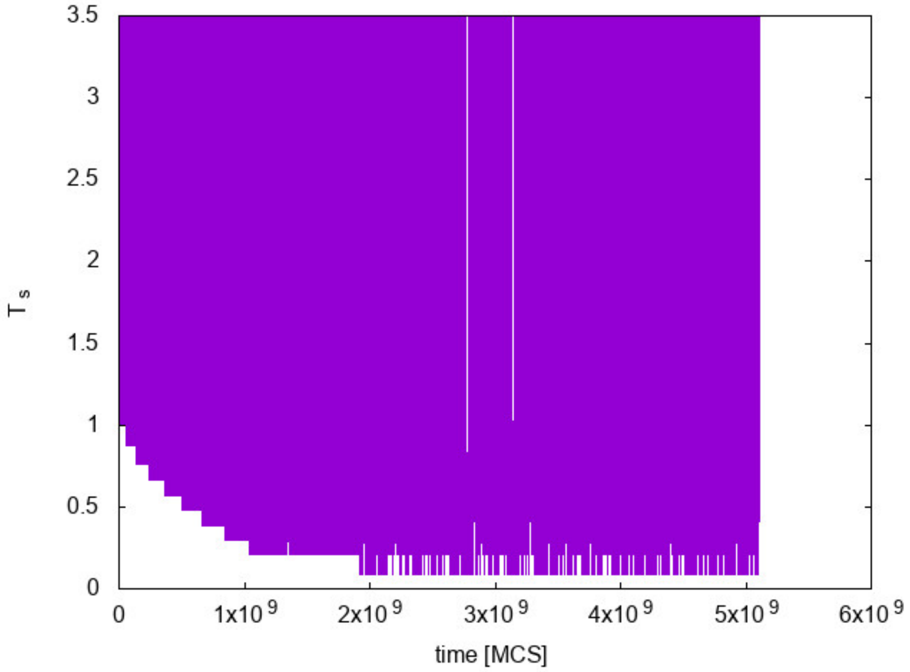


**Figure S1**: the fluctuations in the temperature $T_s$ during a sampling of sequence space with the adaptive simulated tempering of 1BPI.

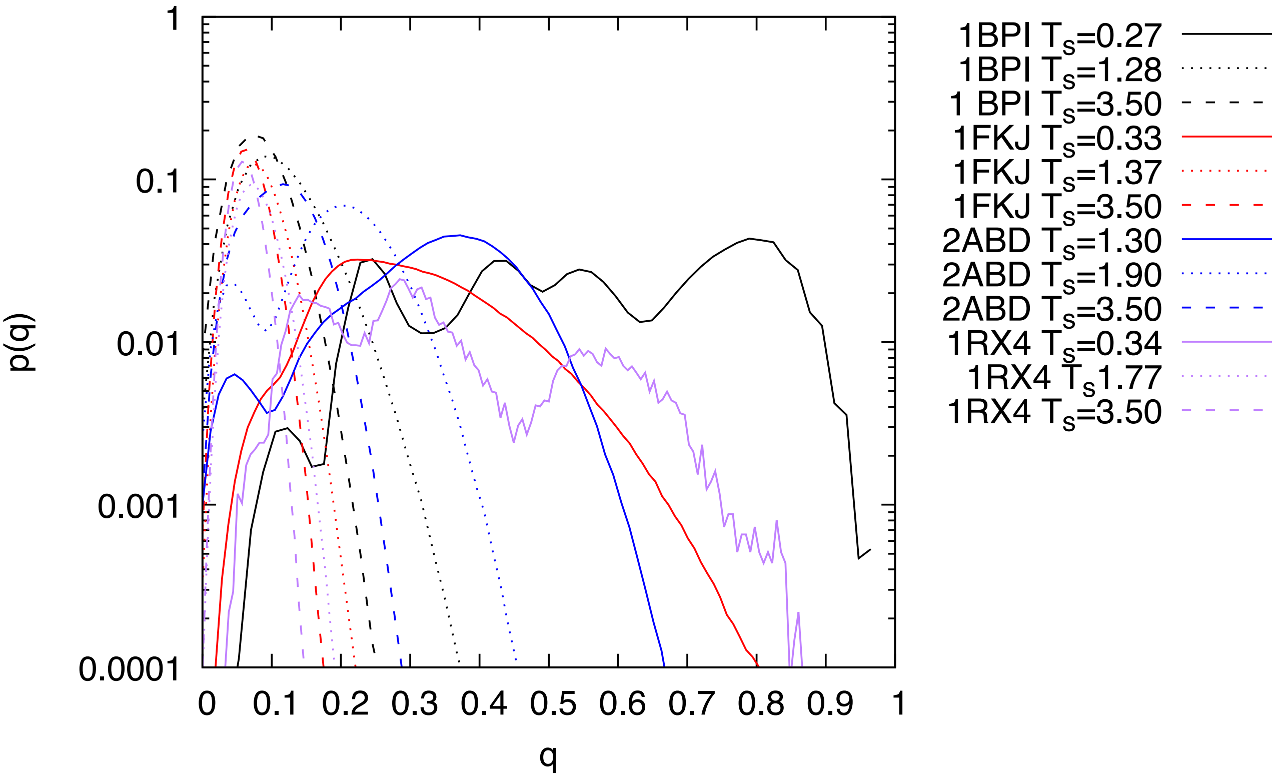


**Figure S2**: The distribution of the Hamming distance $q$ between pairs of sequences in the alignments generated at different temperatures $T_s$ for the various proteins. In the high-temperature and low-temperature phases there is a single peak at low values of $q$. In the frozen phase, $q$ displays a complex distribution which suggests a hierarchical clustering in sequence space, similarly to the behaviour of spin glasses at low temperature.

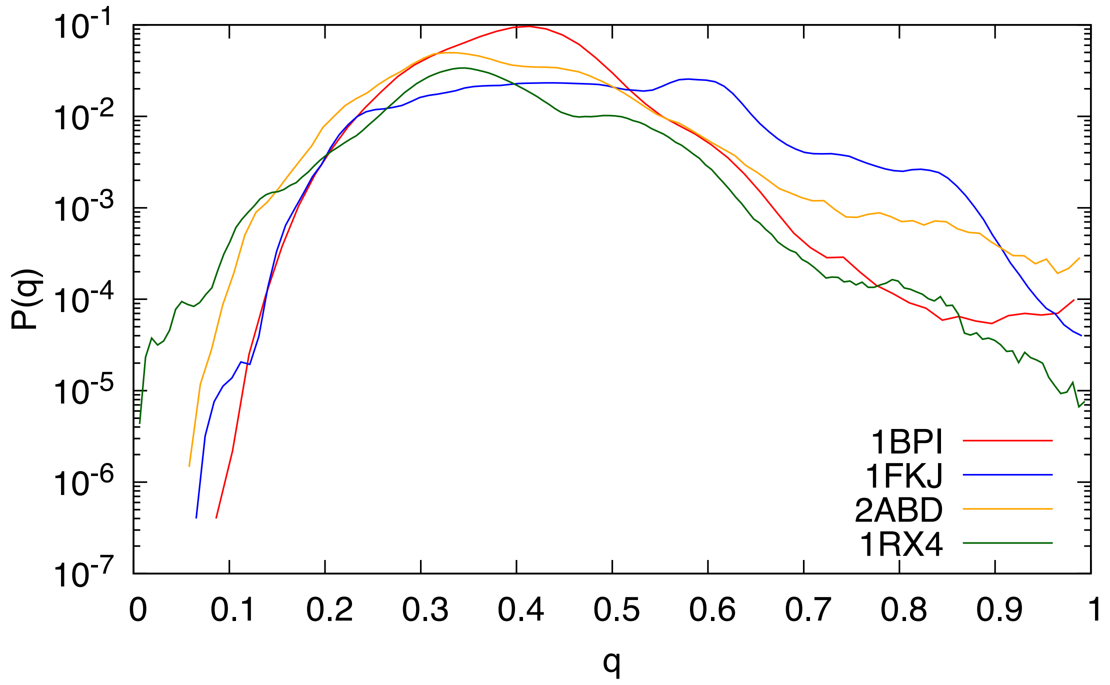


**Figure S3**: The distribution of Hamming distances for the actual alignments of the four proteins.

1BPI 1FKJ

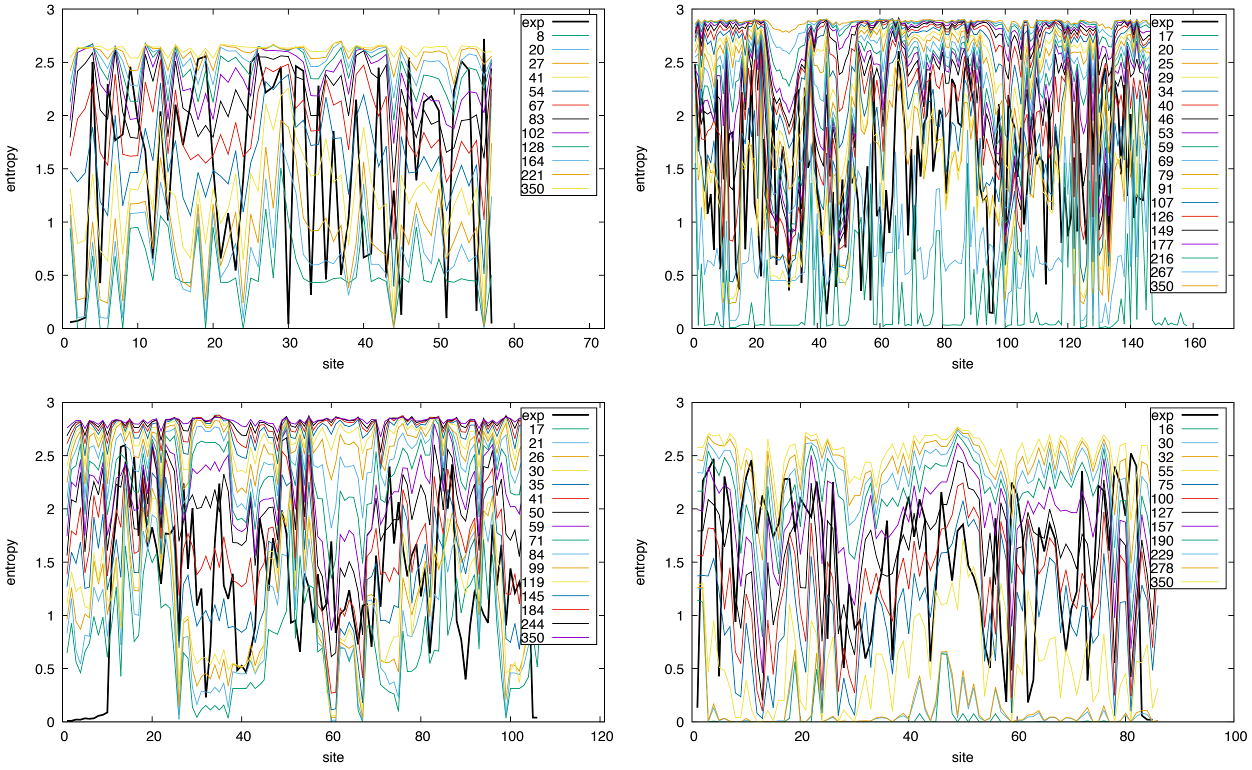


1RX4 2ABD

**Figure S4**: The entropy per site $S_i$ and its distribution for the synthetic alignments generated by the Monte Carlo calculations at different temperatures and for the natural alignments of proteins 1BPI, 1FKJ, 1RX4 and 2ABD.

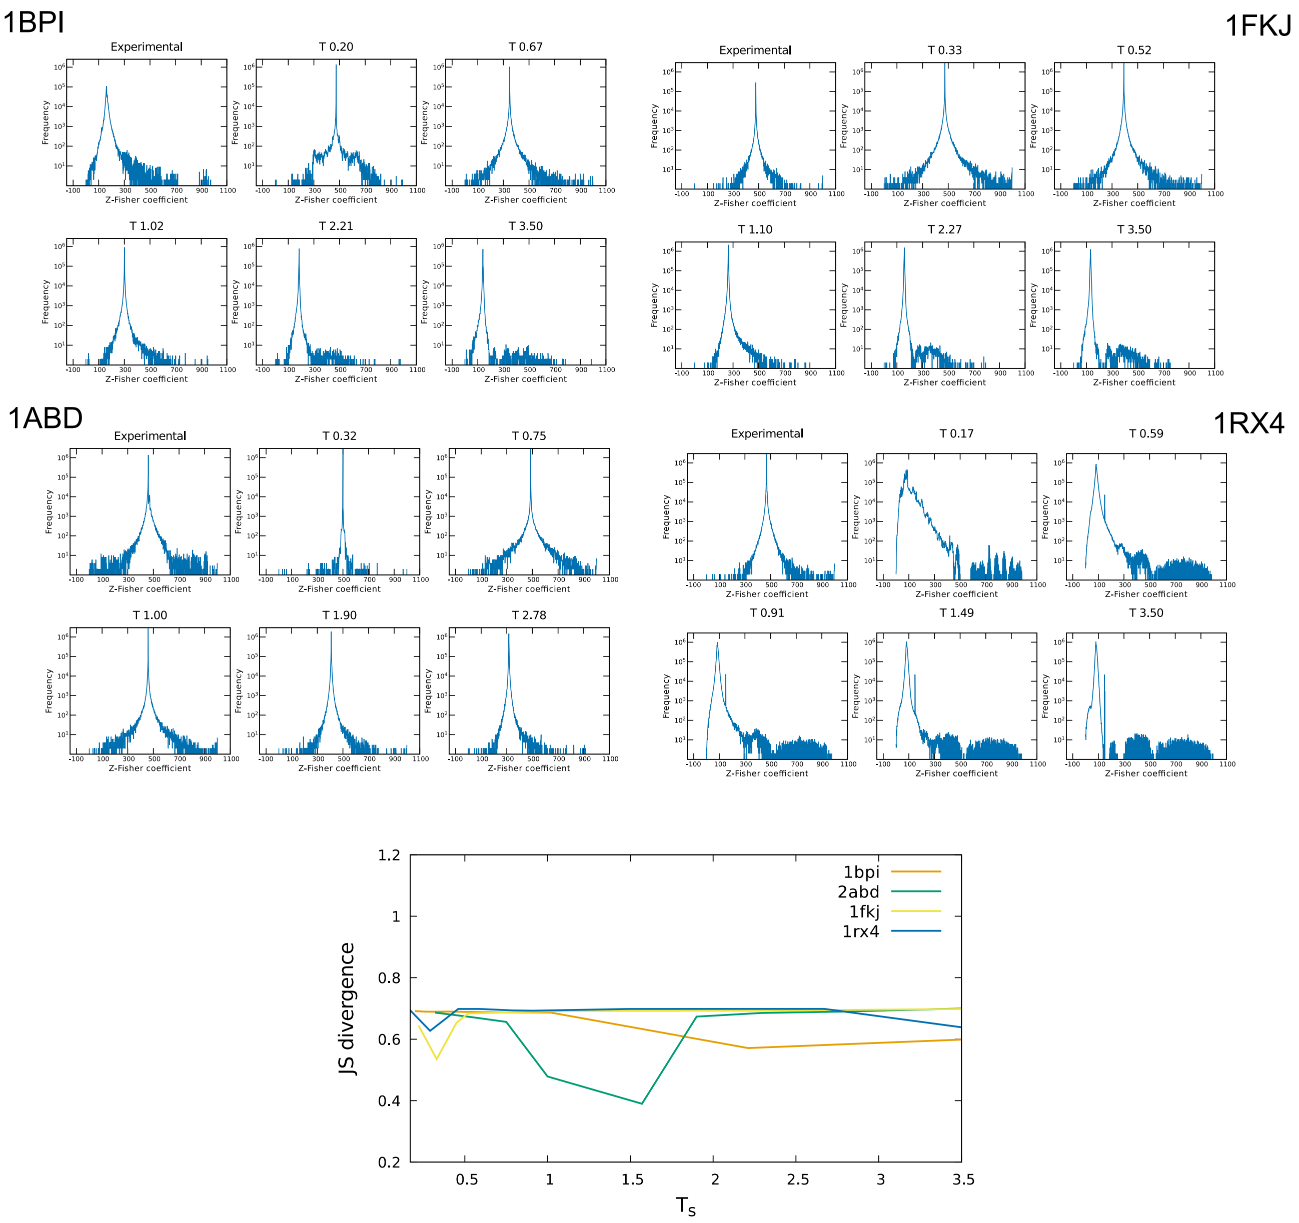


**Figure S5**: The distribution of Fischer-transformed two-point correlation functions $C_{ij}(\sigma_i, \sigma_j)$ calculated for the experimental alignments and for the sequences generated by the model at different temperatures $T_s$ for the four proteins under study. The Fischer transformation is useful for the visualisation because in case of uncorrelated data would give a Gaussian distribution. The bottom plot displays the Jensen-Shannon divergence between the experimental distribution and those obtained at various temperatures.

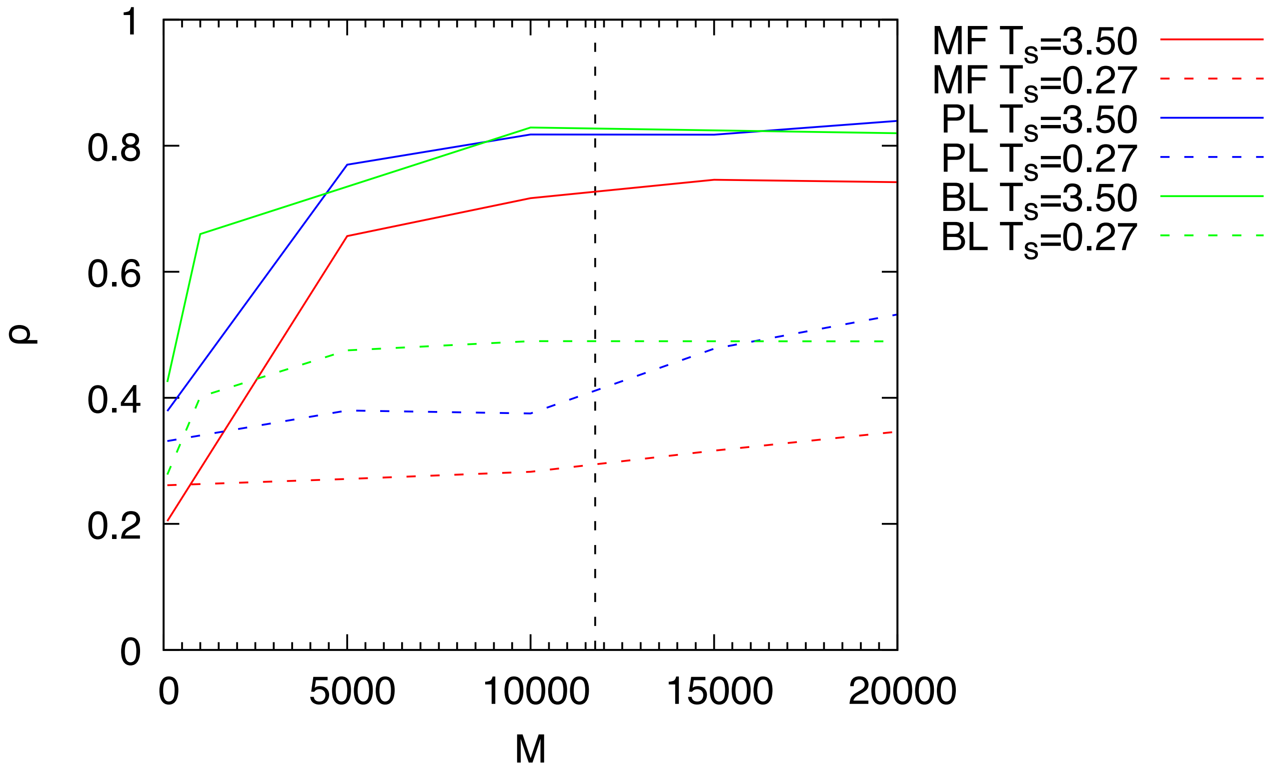


**Figure S6**: The correlation $\rho$ as a function of the number of sequences M for BPI, calculated with the three algorithms at selected temperatures.

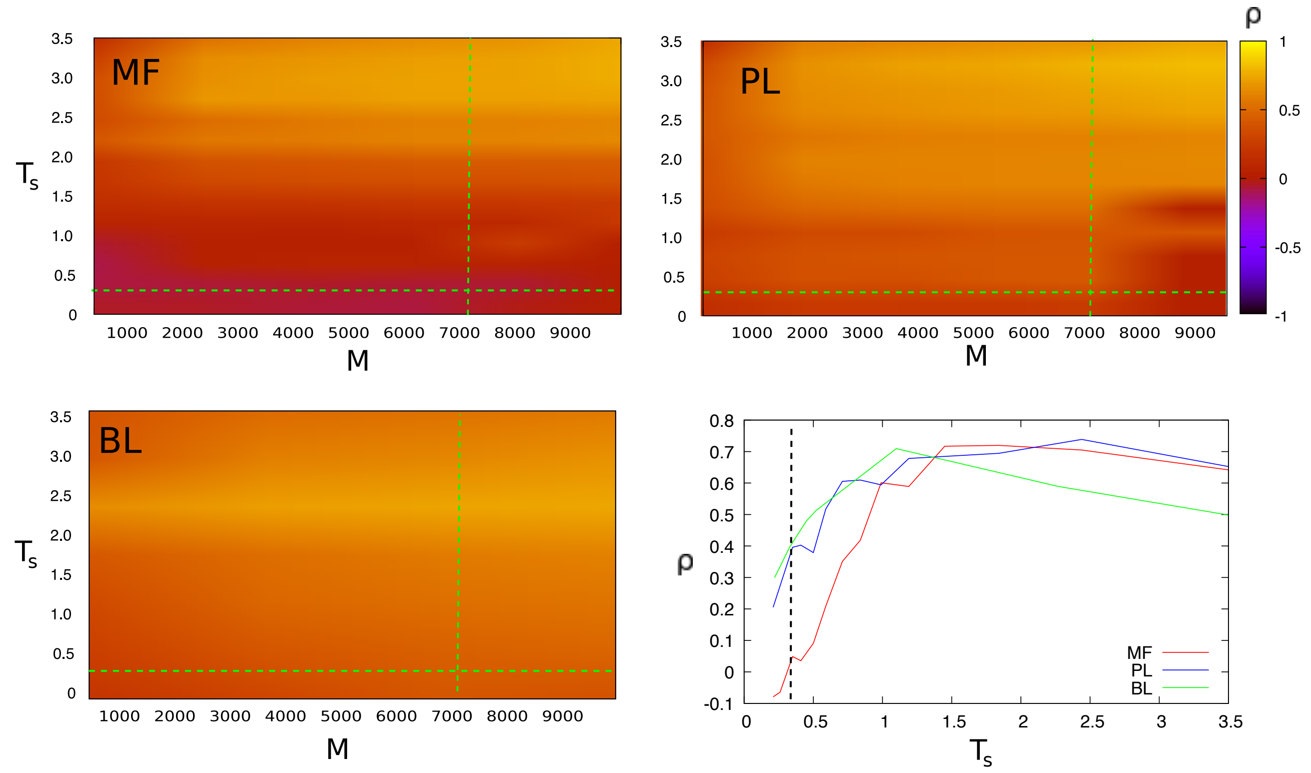


**Figure S7**: Analogously to Fig. 3 of the main text, the Pearson correlation coefficient between the interaction energies used to generate the synthetic sequences and those back-calculated with the mean-field (MF), the pseudolikelyhood (PL) method and the Boltzmann learning method (BL) for protein 1FKJ. Dashed lines indicate the temperature $T_s^n$ and the number of sequences of the true alignment.

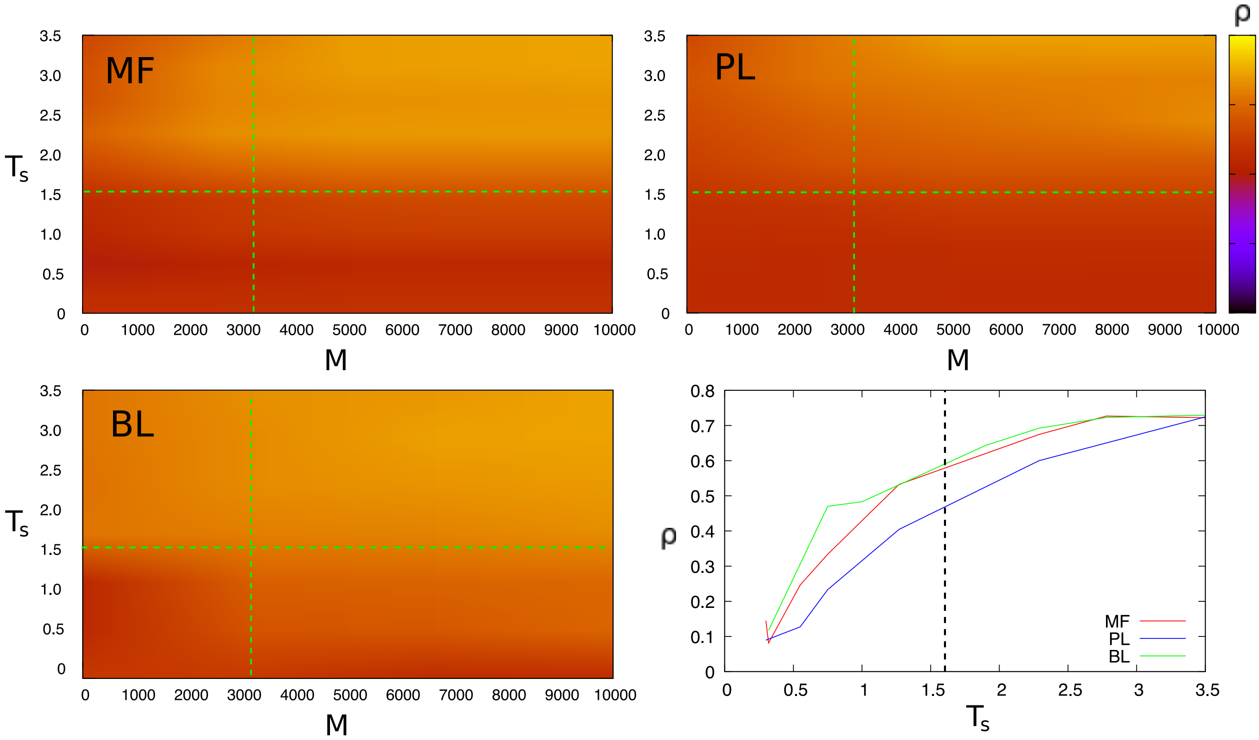


**Figure S8**: same as Fig. S3 for protein 2ABD.

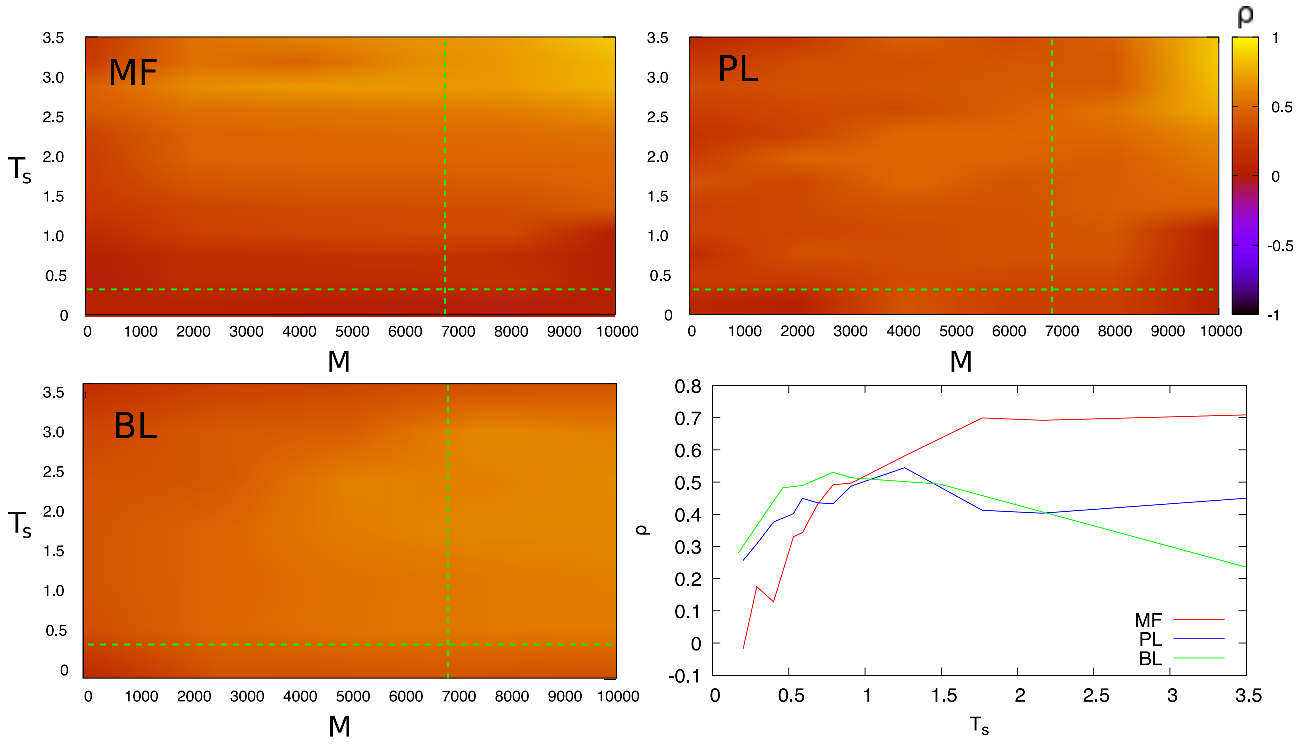


**Figure S9**: same as Fig. S3 for protein 1RX4.

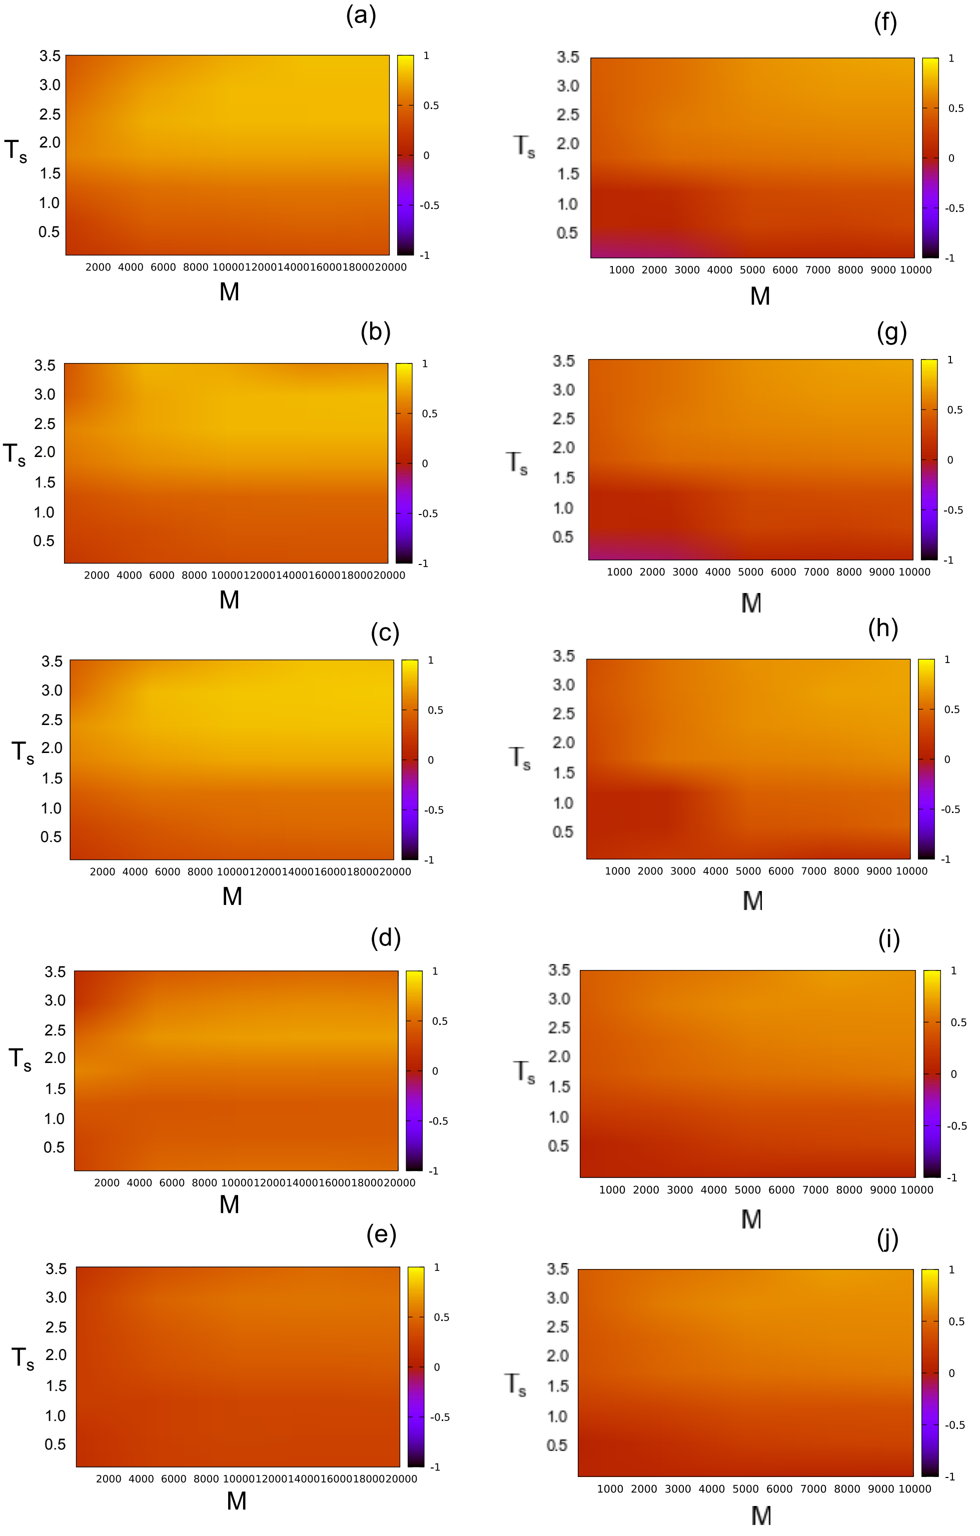


**Figure S10**: the correlation between original and back-calculated energies by BL for 1BPI (a-e) and 2ABD (f-j). The upper six plots (a-c, f-h) are obtained using sequences selected at random from those sampled by the algorithm, and thus can be regarded as “typical” according to the underlying potential; the bottom four plots (d, e, i, j) are obtained using sequences uncorrelated to those sampled.

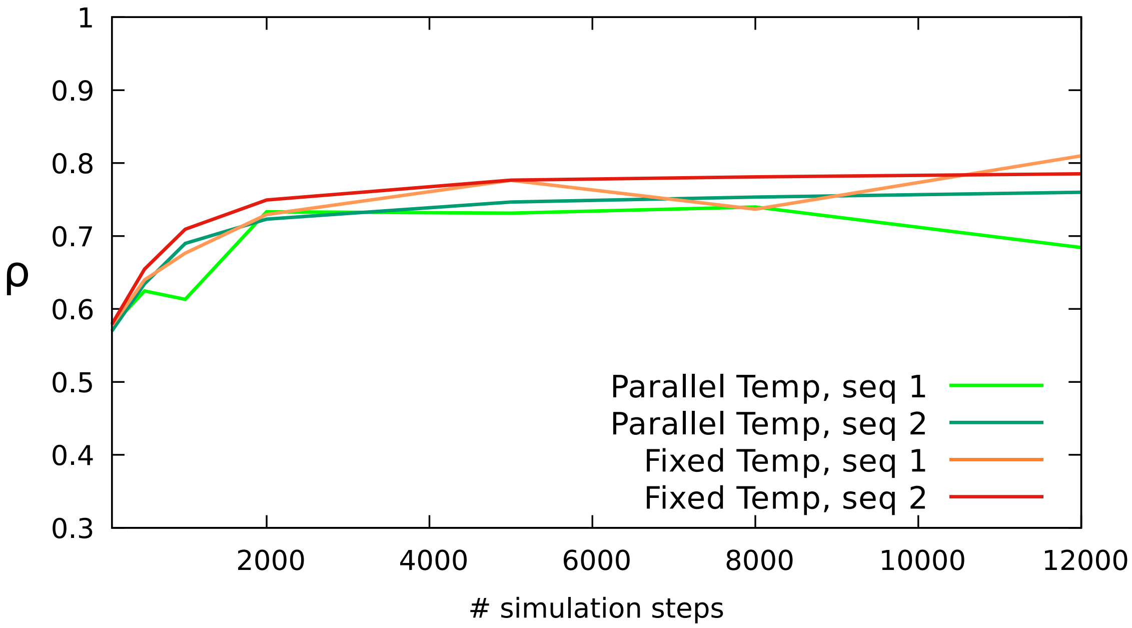


**Figure S11**: The correlation $\rho$ calculated by BL for two sequences of 1BPI at $T_s = 0.5$ as a function of the number of steps of the algorithm (each step is meant as a Monte Carlo attempt at each site of the chain, followed by a step of the steepest-descent in the optimisation of the energies) with the standard implementation described in *Methods* and with a variant in which the sampling of sequence space is carried out with a parallel tempering method DETTAGLI

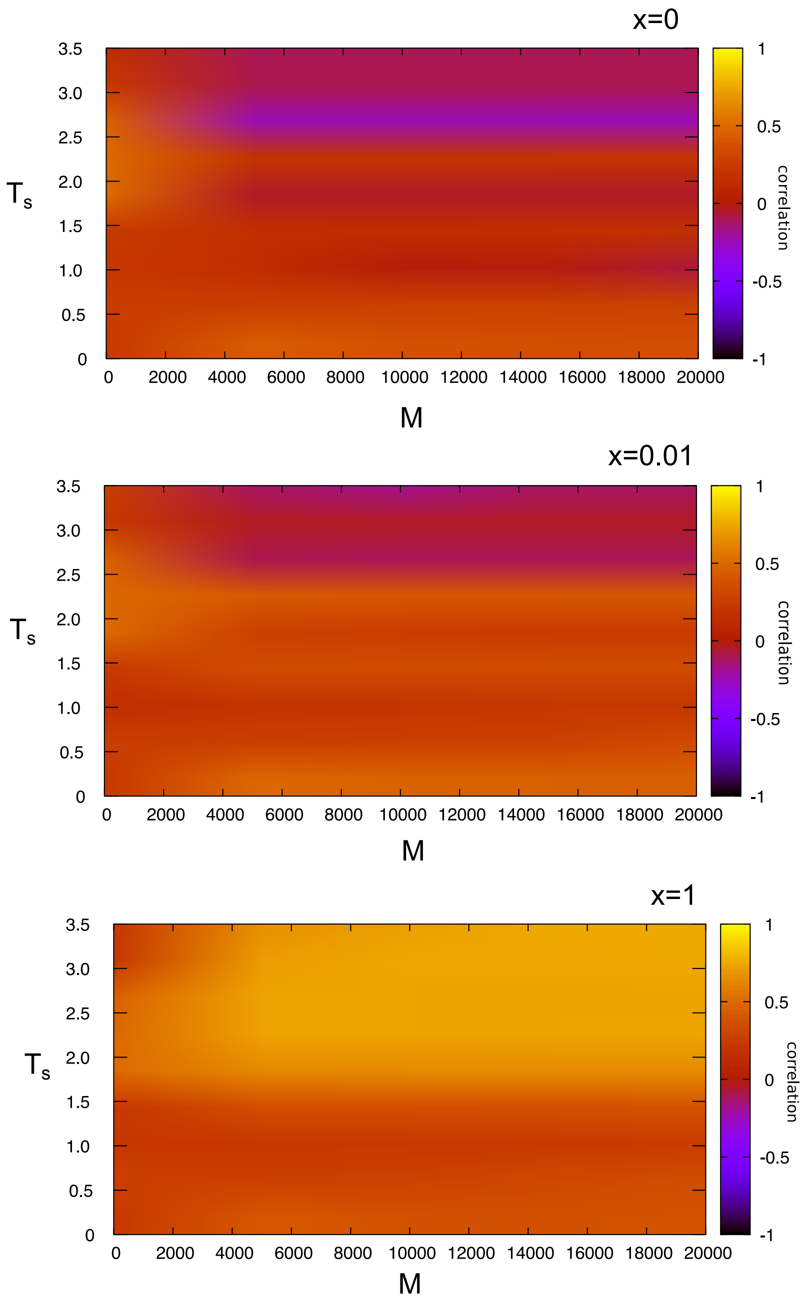


**Figure S12**: The correlation coefficient $\rho$ calculate for 1BPI with the MF algorithm using three different values of the pseudocounts $x$.

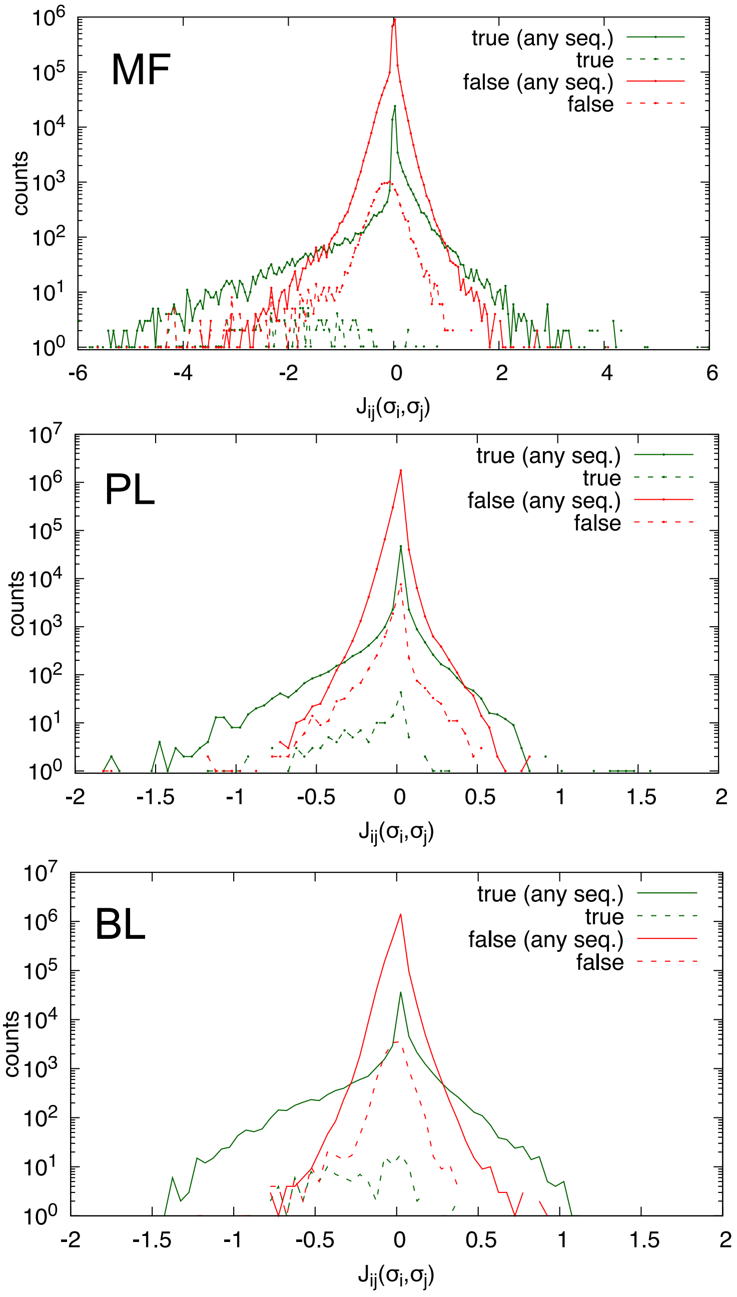


**Figure S13**: The distribution of interaction energies calculated by MF, PL and BL for 1FKJ at $T_s = T_s^n$ for the true native contacts (solid green curve) and for the non--native contacts (solid red curve). The dashed curves indicate the distribution of native and non--native energies associated only to a "typical" sequence (cf. Fig. S8).

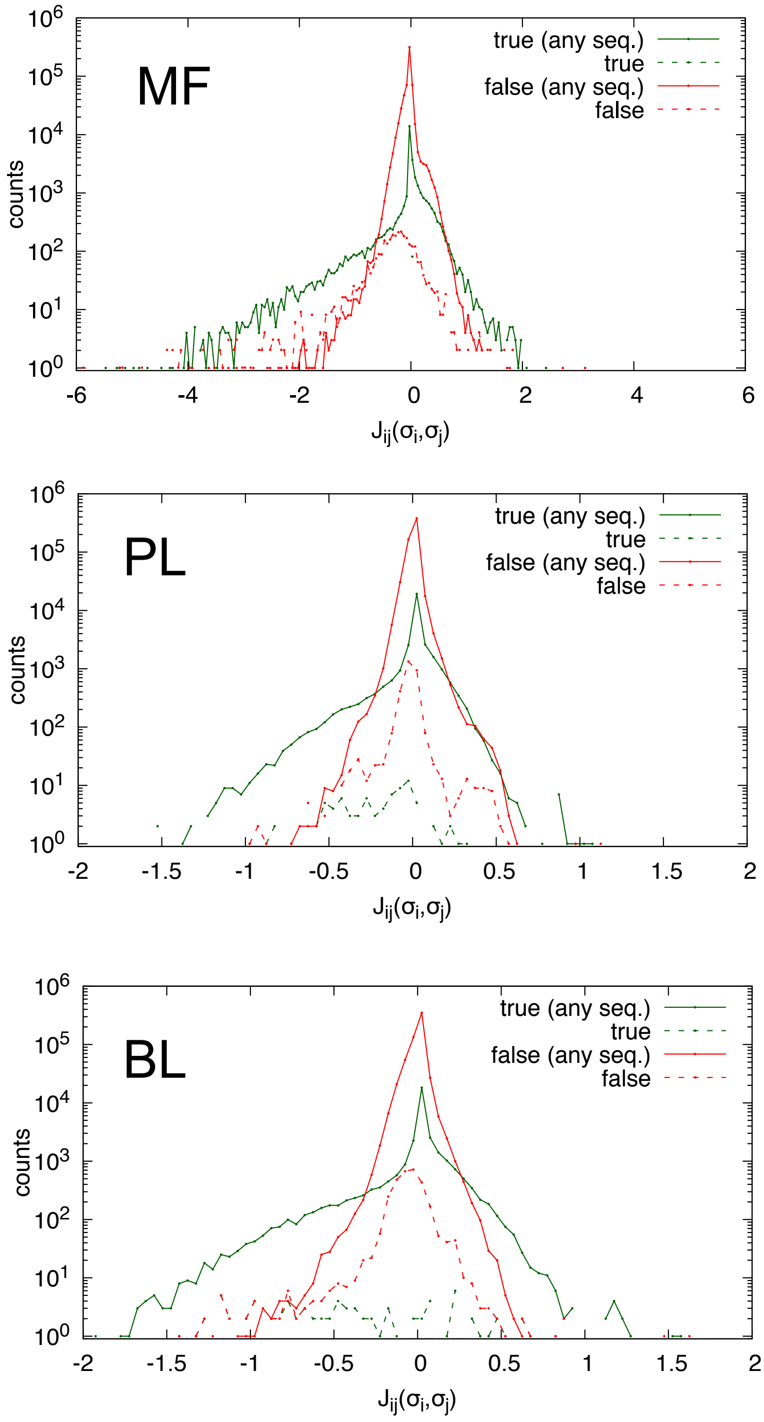


**Figure S14**: The distribution of interaction energies calculated by MF, PL and BL for 1BPI (analogously to Fig. 5 in the main text), calculated at $T_s = 102$.

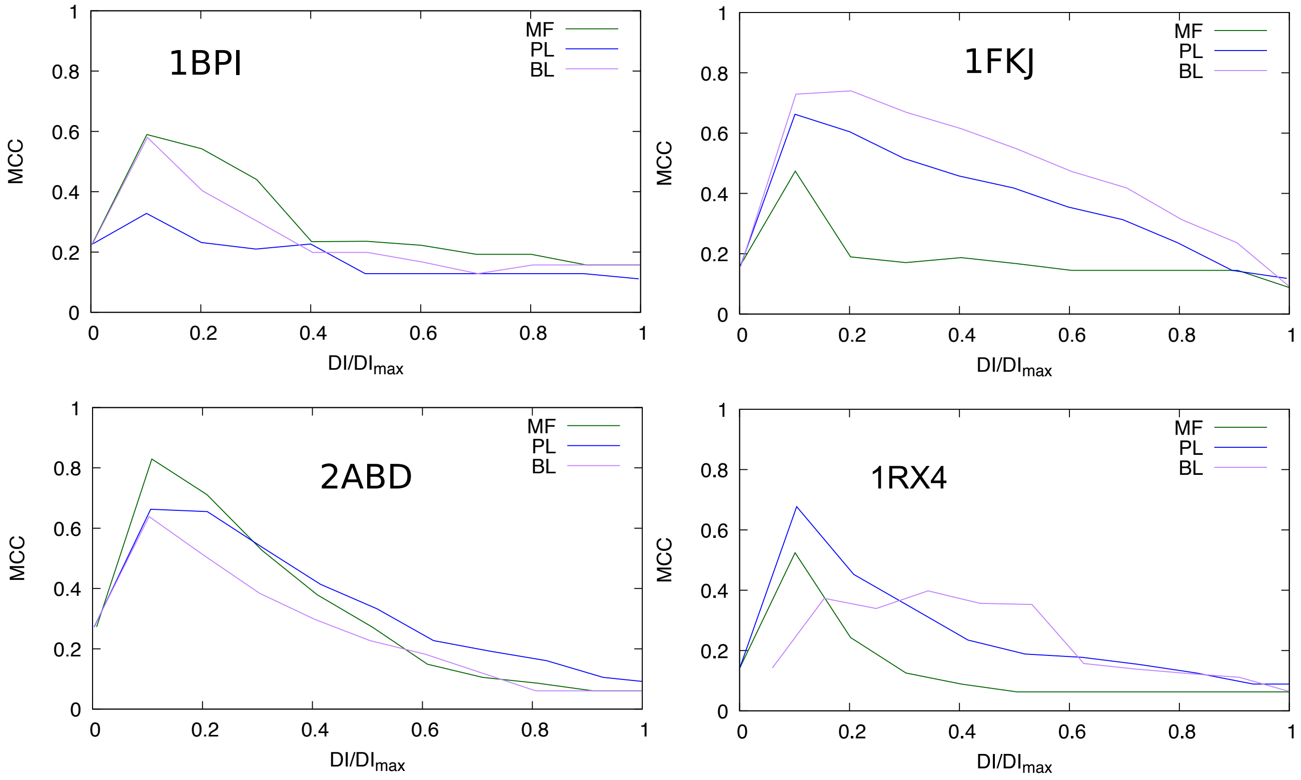


**Figure S15**: The MCC associated with sequences generated at $T_s^n$ with the three algorithms, as a function of the threshold on the relative direct information.

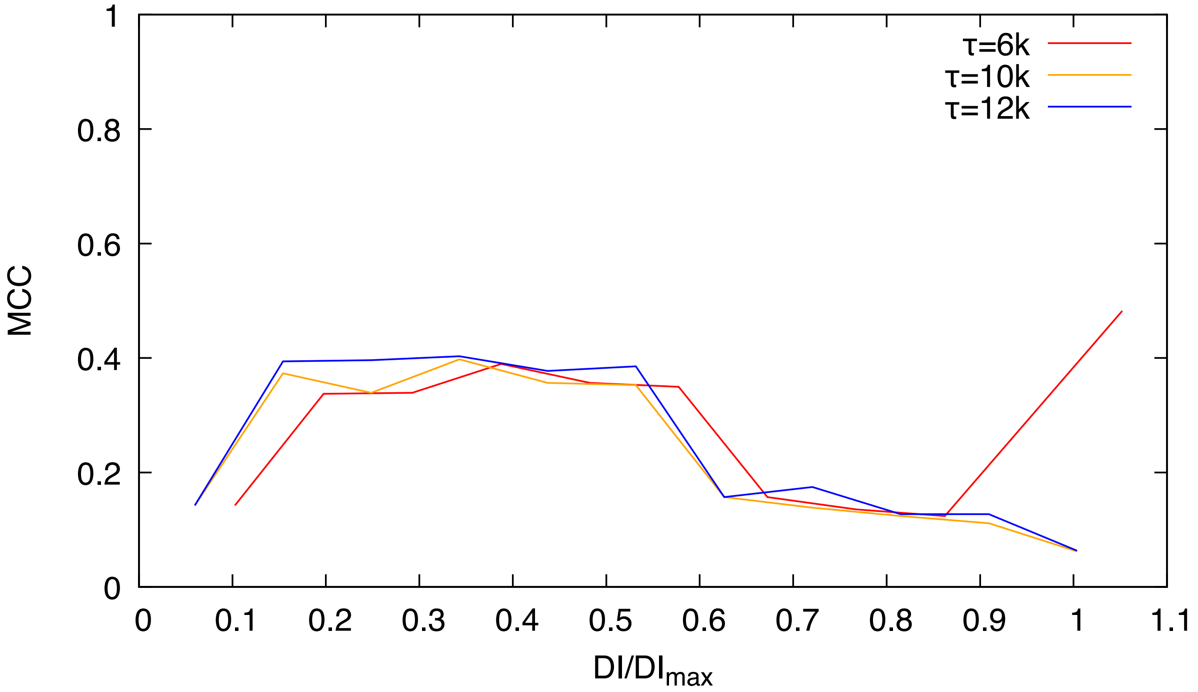


**Figure S16**: The MCC of 1RX4 at $T_s = T_s^n$ calculated with BL using different values of $\tau$, and consequently different length of the optimisation of the parameters.

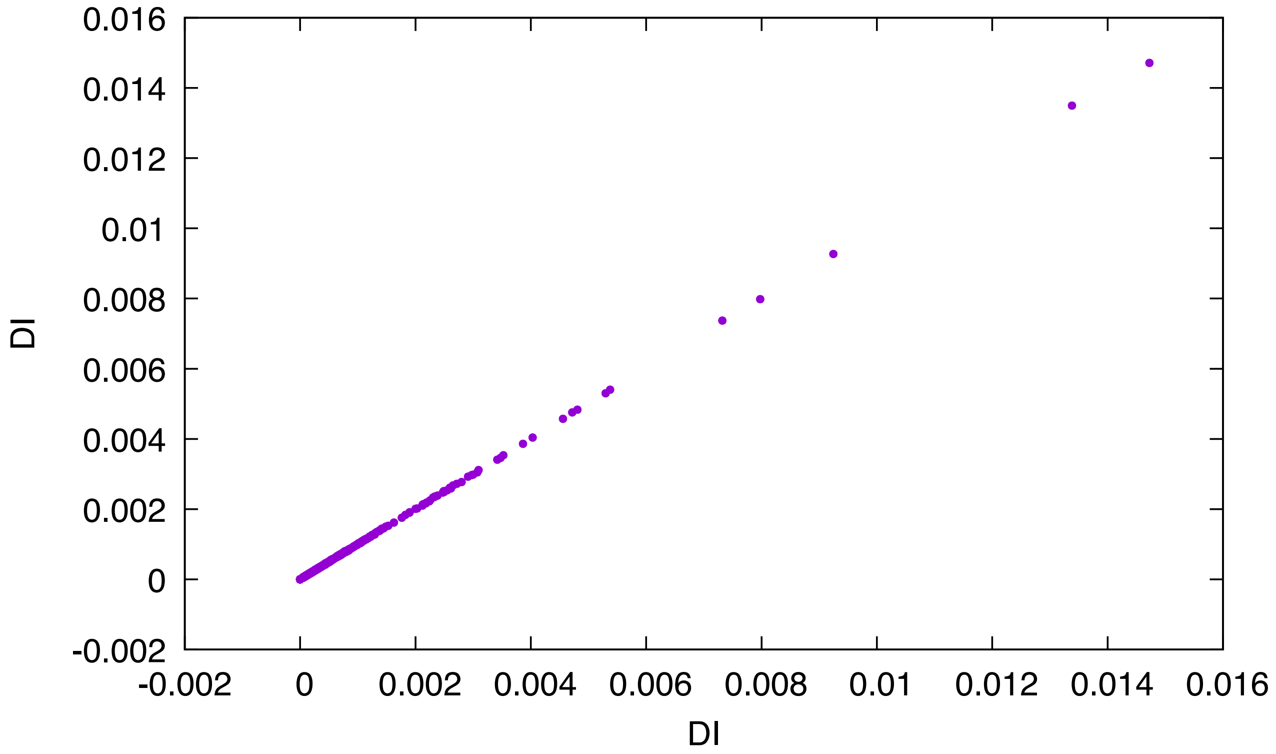


**Figure S17**: Direct information (DI) predicted for 1BPI at $T_s = T_s^n$ in two independent optimisation runs of BL.

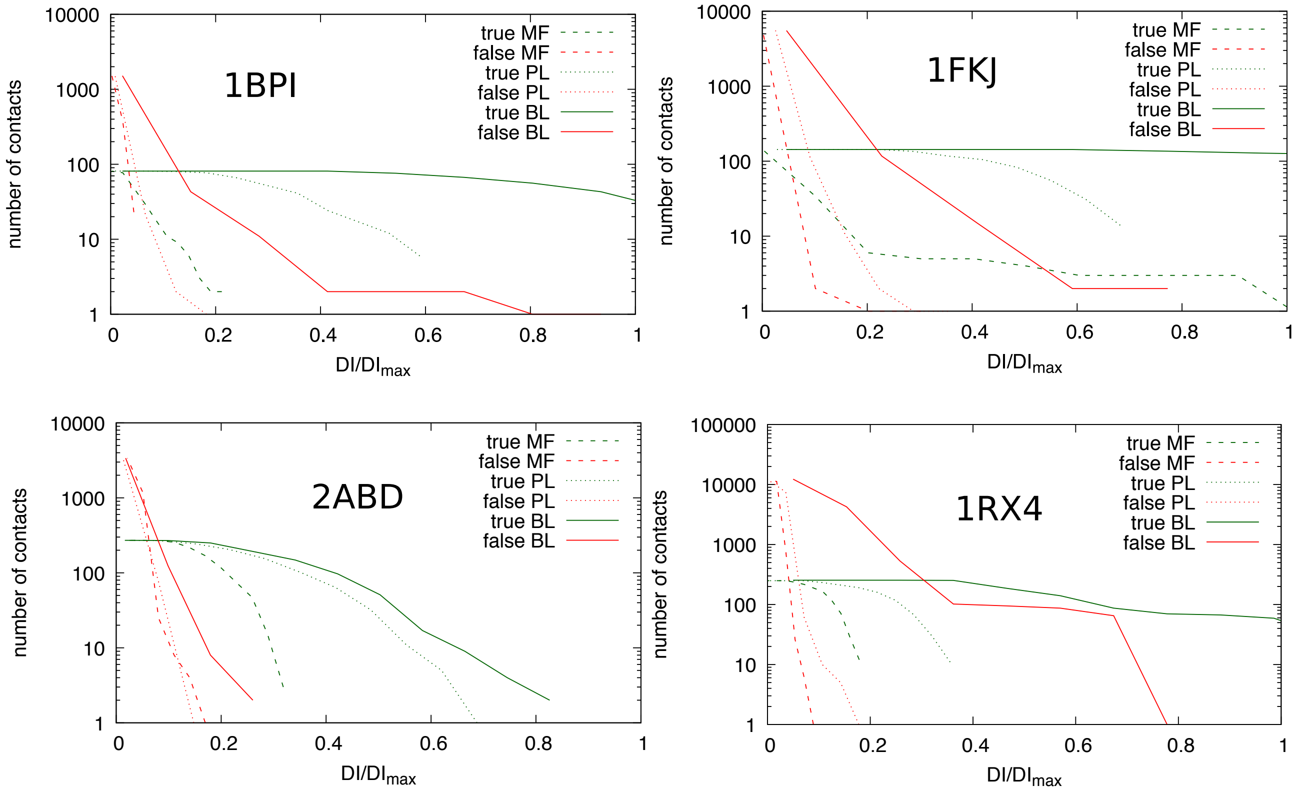


**Figure S18**: The number of native and non-native contacts obtained from direct information, as a function of the threshold at $T_s = 1$ for 1BPI, 1FKJ and 1RX4 and $T_s = 2$ for 2ABD, that is in the low-temperature, non-glassy phase.

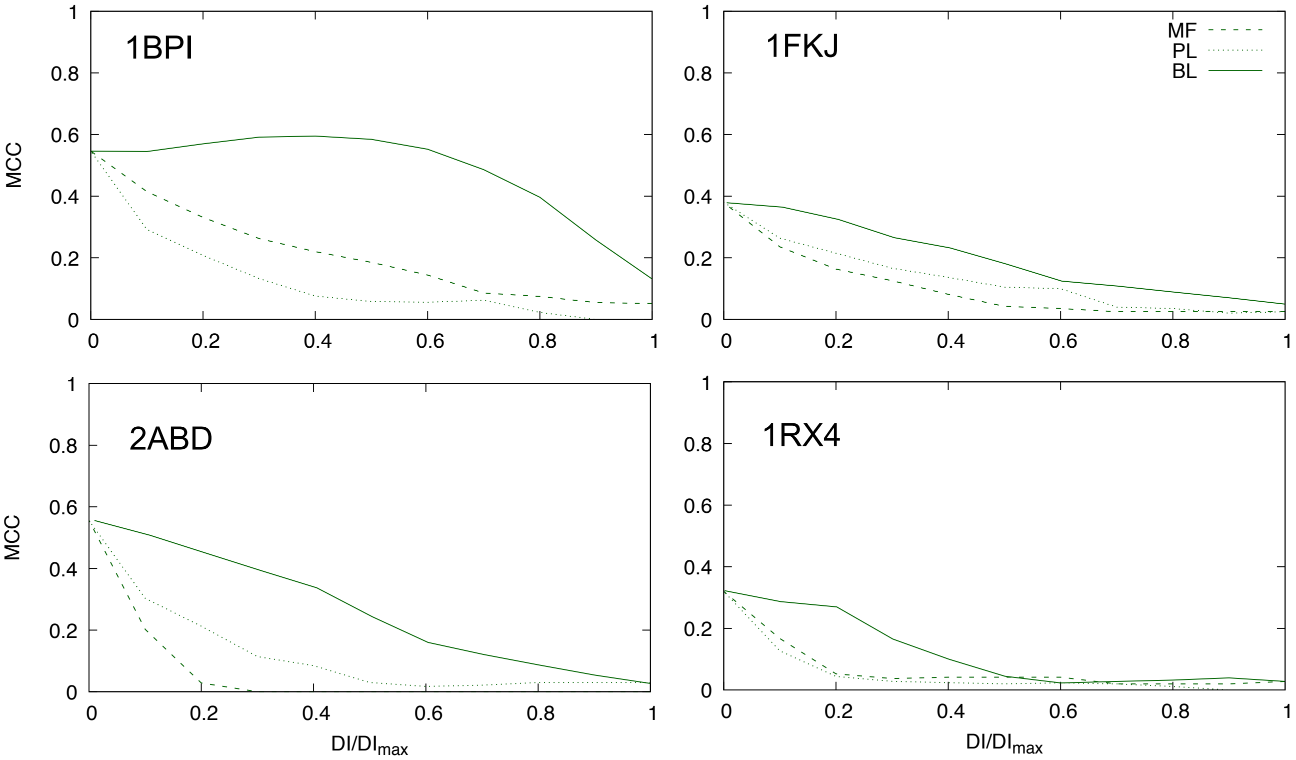


**Figure S19**: The MCC for the real alignment of the four proteins.

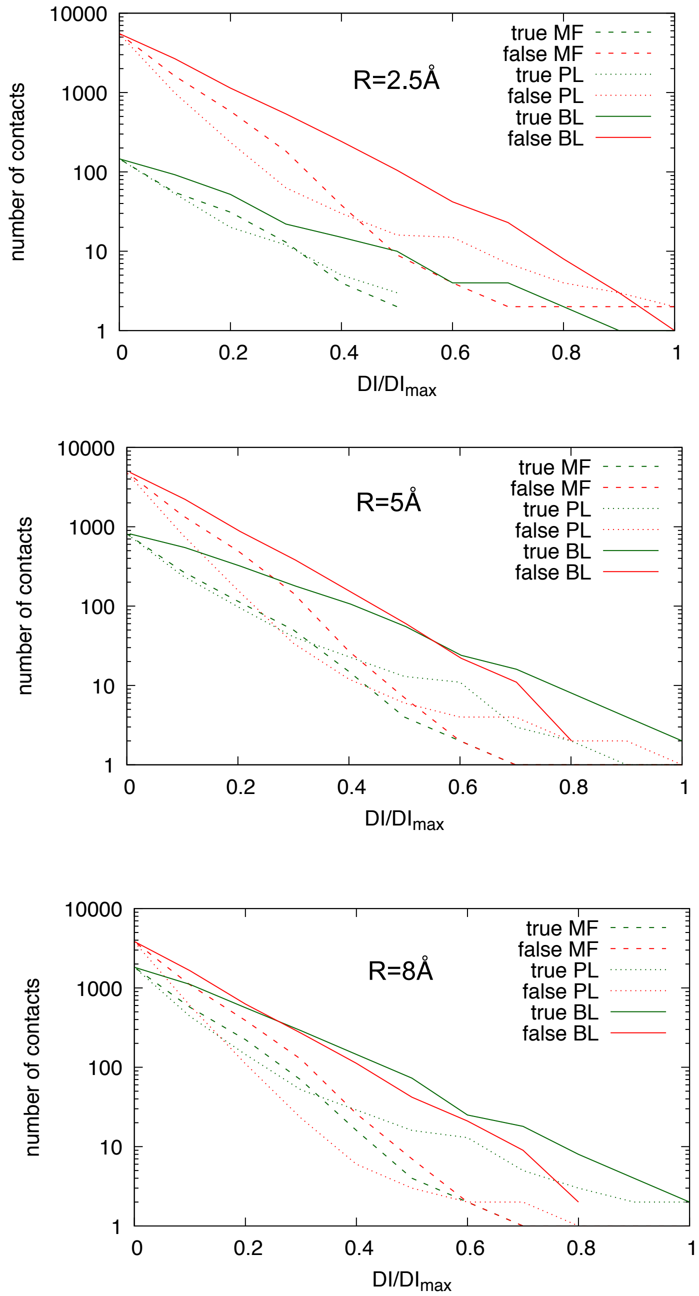


**Figure S20**: The dependence of the results on 1FKJ on the threshold length R used to define a contact in the crystallographic conformation.
